# Supplementary material for: Dimensional Crossover Tuned by Pressure in Layered Magnetic NiPS3
Source: arXiv:2009.14051 source file (2020-09-29)
Supplement: Supplementary file 1 [file Supplementary_Material_of_NiPS3.pdf]

# Supplementary Material

(1) Pressure dependence of Raman spectra of bulk $NiPS_3$

Raman scattering is more sensitive to structural changes. In order to verify the phase transition of $NiPS_3$, we conducted a Raman scattering study of bulk $NiPS_3$ under pressure. Fig. S1 is the Raman spectra of bulk $NiPS_3$ under different pressures. From these data, we can see that there is a new peak occurs around 15 GPa, so there is a phase transition begins to appear. According to previous experiments and calculation results [1,2], this new peak does not appear out of nowhere. This phonon already exists in the structure with space group C2/m, but it was not observed at low pressure due to weak signals or other reasons. When the pressure is increased to 15 GPa, the unit cell parameters are abruptly changed, and the Raman tensor is also changed. So that the intensity of this phonon is changed. Therefore, under the pressure of 15 GPa, an isostructural phase transition occurs. This result is consistent with the results of high-pressure XRD and theoretical simulations. However, since the intensity of the peaks above 27 GPa is very small, phase transition above 27 GPa is not observed.

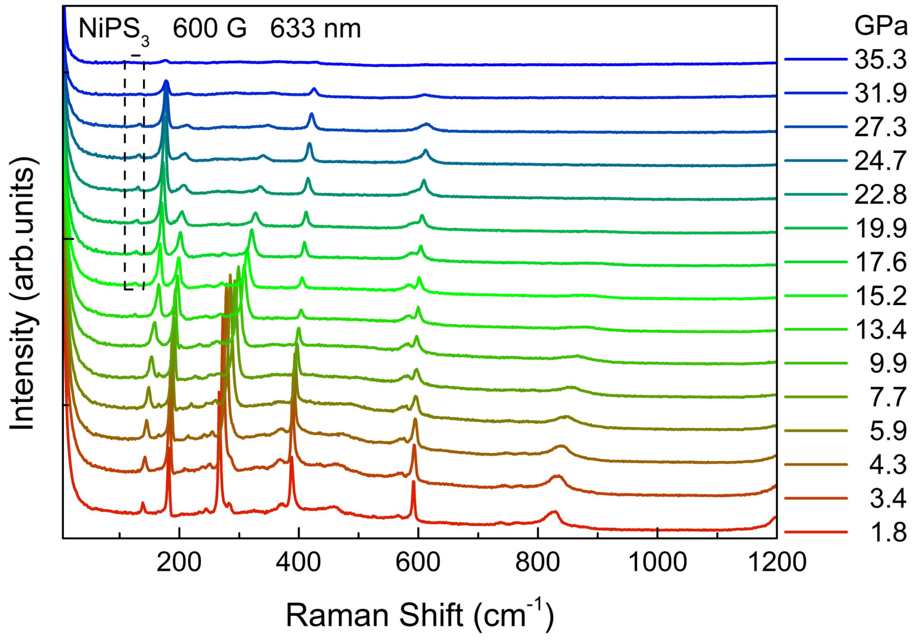


Fig. S1 Pressure dependence of Raman spectra of bulk $NiPS_3$ from 1.8 GPa to 35.3 GPa.

(2) Optic reflection pictures of bulk $NiPS_3$ under different pressures

We got optic reflection pictures of bulk $NiPS_3$ under different pressures by only turning on the top light source. From Fig. S2, we can see that the sample begins to show a little metallic luster around 22.4 GPa, and the whole sample has a very obvious metallic luster above 27.3 GPa. So the sample started to metallize around 22 GPa. The result is consistent with the data of resistance and infrared measurements.

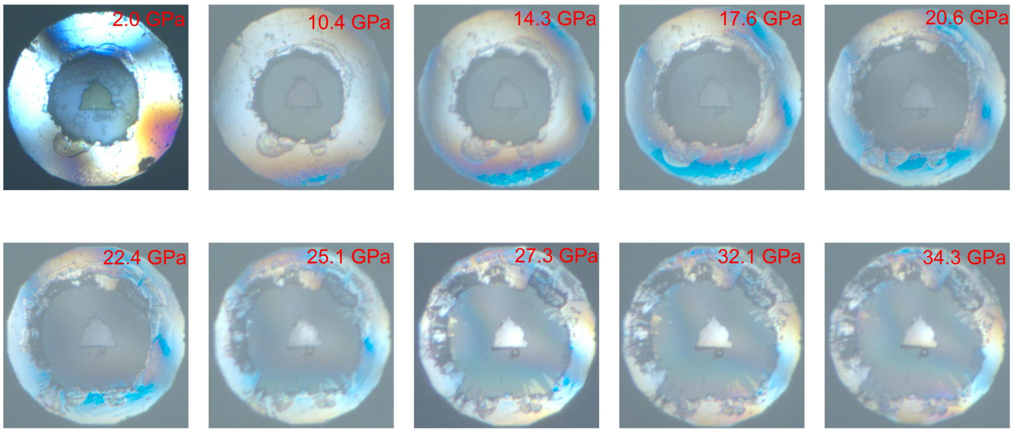


Fig. S2 Optic reflection pictures of bulk $NiPS_3$ under different pressures. Only the top light source is turned on when taking photos.

(3) The temperature dependence of the resistance under different pressures

The temperature dependence of the resistance of bulk $NiPS_3$ under different pressures is plotted in Fig. S3. From Fig. S3(a) we can see that at the lower-pressure 14.2 GPa, data still show the activated behavior of an insulator, similar to the ambient pressure data. But increasing pressure drastically decreases the magnitude of the resistance. At pressures above 20.2 GPa the resistance begins to decrease with decreasing temperature — indicative of metallic behavior [Fig. S3(b)]. In the higher-pressure data shown in Fig. S3(c), resistance continues to decrease and the metallic resistance is still observed. The resistance of bulk $NiPS_3$ has been reduced by several orders of magnitude over the entire pressure range.

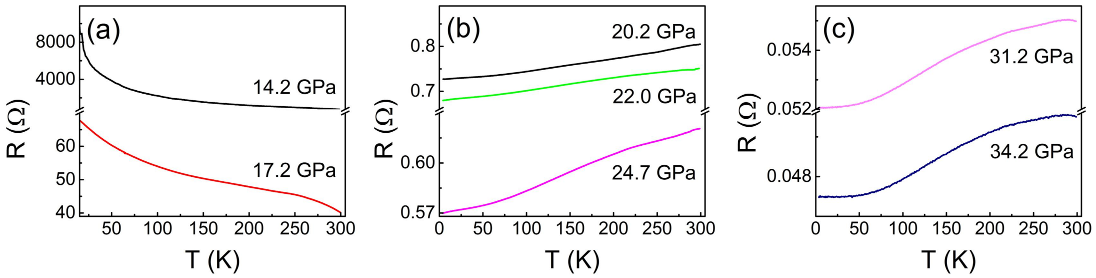


Fig. S3 Resistance of bulk $NiPS_3$ plotted against temperature, at pressures from 14.2 GPa to 45.1 GPa. The resistance is drastically suppressed with applied pressure.

(4) Changes of two-magnon signal with temperature in different channels

Temperature-dependent Raman scattering measurements of bulk $NiPS_3$ carried out from 5.6 to 300 K [Fig. S4(a)]. Fig. S4(b) and (c) display the temperature-dependent of Raman spectra of bulk $NiPS_3$ in parallel and cross-polarization configurations from 5.6 to 300 K at ambient pressure. From Fig. S4(a), (b) and (c) we can see that a broad peak centered at ~550 $cm^{-1}$ appears in the antiferromagnetic phase due to two-magnon scattering. From these data, we can observe that the two-magnon signals gradually grow and shift towards higher frequencies as the temperature decreases below the antiferromagnetic phase transition temperature ($T_N$). These phenomena are typical of antiferromagnetic materials.

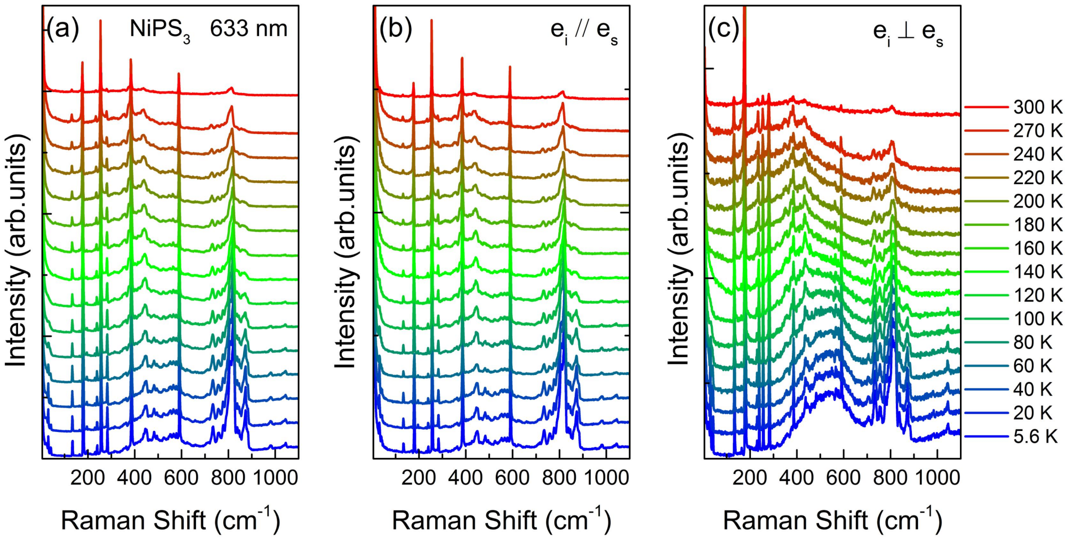


Fig. S4 (a) Temperature dependence of Raman spectra of bulk $NiPS_3$ from 5.6 to

300 K at ambient pressure; (b) Temperature dependence of Raman spectra of bulk $NiPS_3$ in parallel-polarization configuration from 5.6 to 300 K at ambient pressure; (c) Temperature dependence of Raman spectra of bulk $NiPS_3$ in cross-polarization configuration from 5.6 to 300 K at ambient pressure.

(5) The behavior of the two-magnon with pressure at 5 K

Fig. S5(a) and (b) are the Raman scattering of bulk $NiPS_3$ in no-polarization and parallel-polarization configuration under different pressures at 5 K. From Fig. S5(a) and (b) we find that the behavior of the two-magnon with pressure is the same as that of Fig. 4(a). The two-magnon signal was gradually suppressed and shift towards higher frequencies as the pressure increased. And the two-magnon signal was totally suppressed around 27 GPa. We also fitted the data in Fig. S5(a) and (b) and got the two-magnon areas of bulk $NiPS_3$ in no-polarization and parallel-polarization configuration under different pressures [Fig. S5(c)]. From Fig. S5(c), we can see that the area of the two-magnon decreases with increasing pressure and the magnetism completely disappears at 27 GPa. The same behavior as Fig. 4(b).

In addition to the change of the two-magnon with pressure, we also found some changes in the phonons. When the pressure is higher than 15.2 GPa, it was found that one of the $A_g$,$B_g$ phonon modes was split [Fig. S5(d)], so a phase transition may occur under this pressure. However, since the $A_g$ and $B_g$ phonon modes of the bulk $NiPS_3$ are degenerate, this peak may not be split, but because the $A_g$ and $B_g$ modes are separated with pressure changes. For the abnormal change of this phonon, we need to make further exploration to discover the cause of this phenomenon.

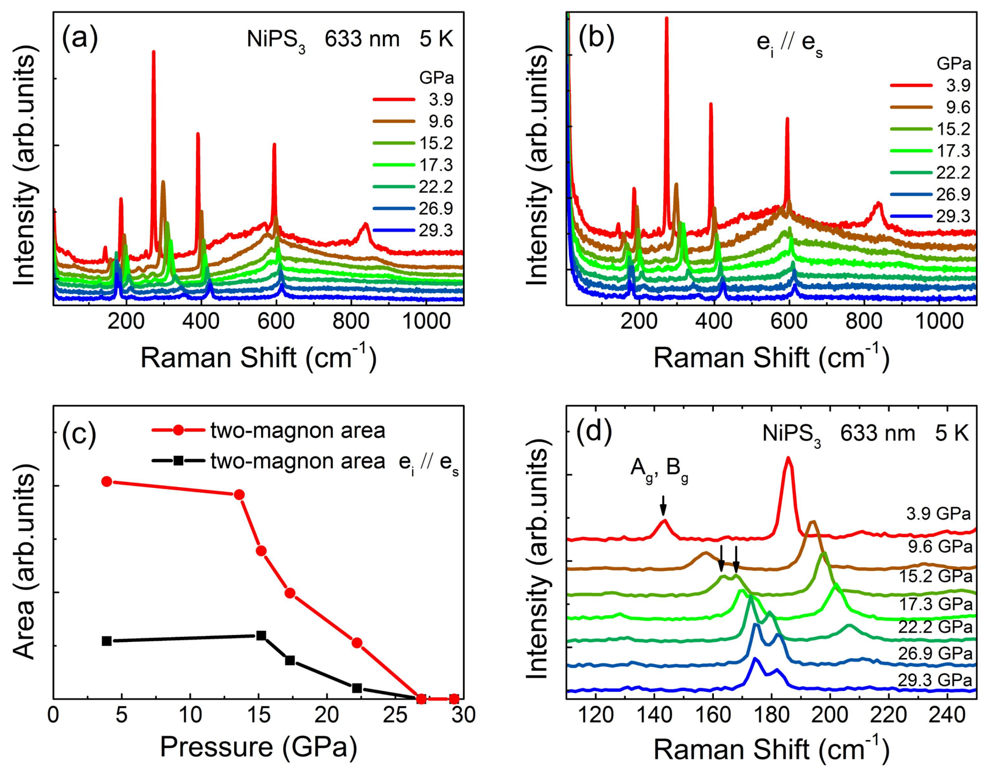


Fig. S5 (a) Raman scattering of bulk $NiPS_3$ under different pressures at 5 K; (b) Raman scattering of bulk $NiPS_3$ in parallel-polarization configuration under different pressures at 5 K； (c) Two-magnon areas of bulk $NiPS_3$ in no-polarization and parallel-polarization configuration under different pressures, the data points in (c) are extracted from Raman spectra in (a) and (b); (d) Raman scattering from 80 $cm^{-1}$ to 250 $cm^{-1}$ of bulk $NiPS_3$ under different pressures at 5 K.

(6) The behavior of the two-magnon with pressure at different temperatures

we conducted the Raman measurements of bulk $NiPS_3$ in different configurations under different pressures at different temperatures, see Fig. S6. From these data we can find that the two-magnon signal was gradually suppressed and shift towards higher frequencies as the pressure increased. Such a rule is consistent with Fig. 4(a).

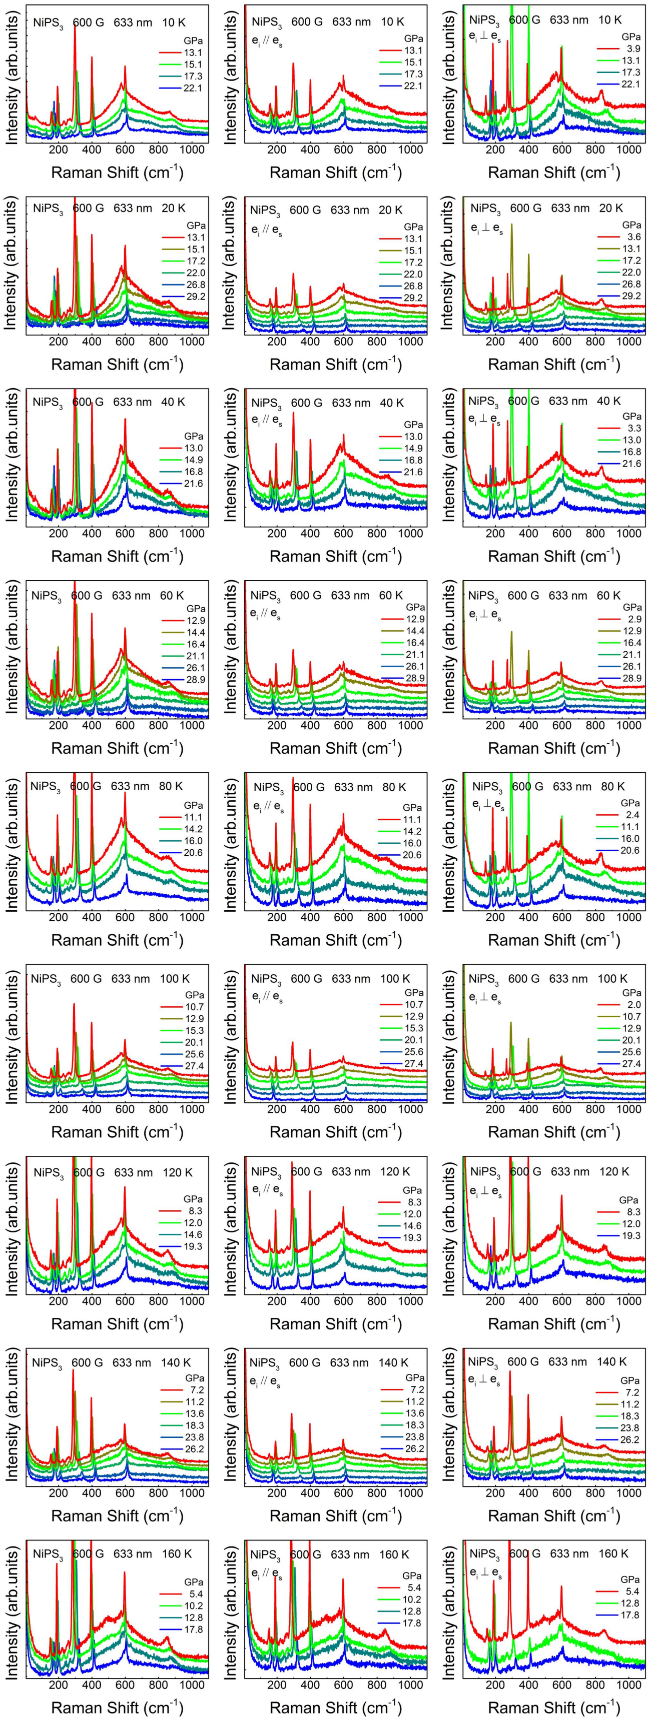


Fig. S6 Raan spectra of bulk $NiPS_3$ in different configurations under different pressures at different temperatures.

(7) DOSs for bulk and monolayer $NiPS_3$

The total and projected electronic density of states (DOS) at 20 GPa can be seen in Fig. S7. As shown in Fig. S7(a), the bulk $NiPS_3$ at 20 GPa shows a metallic behavior. The states around the Fermi level are mainly contributed by the Ni-*3d* and S-*2p* states. Meanwhile, the splitting between the spin-up and spin-down DOS peaks below the Fermi level for the Ni-*3d* states results a moment of 0.54 $\mu_B$ on Ni sites. For comparison, we have also calculated the total and projected electronic DOSs at 20 GPa for the monolayer $NiPS_3$. As shown Fig. S7(b), the monolayer $NiPS_3$ shows a semiconducting behavior with a band gap of 0.43 eV. The states near the Fermi level are mainly contributed by the Ni-*3d* and S-*2p* states like as the bulk $NiPS_3$, while the bandwidth of the Ni-*3d* and S-*2p* states are strongly narrowed in contrast with their bulk DOSs, and show a larger splitting between the spin-up and spin-down DOS peaks below the Fermi level for the Ni-*3d* states, which results a larger moment of 0.80 $\mu_B$ on Ni sites. These results suggest the magnetic moments and electronic property (metallic or semiconducting) are strongly correlated with the interlayer distance.

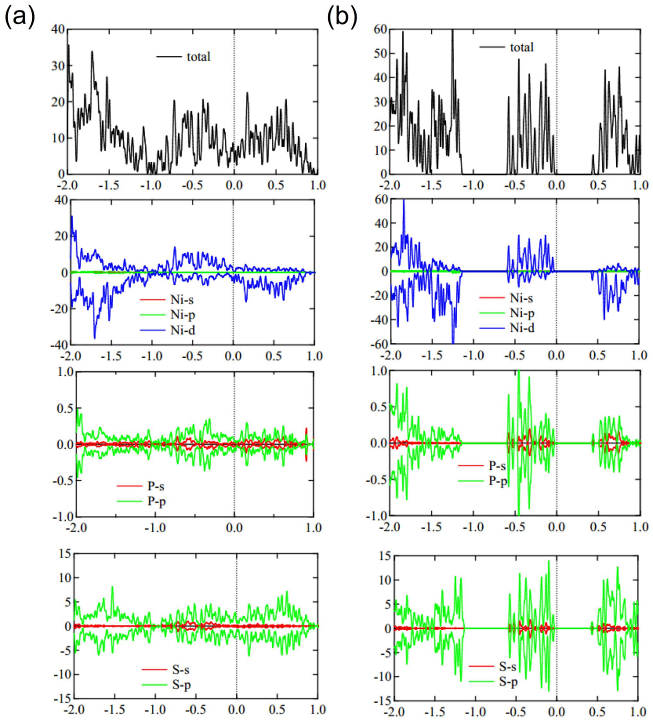


Fig. S7 Total and partial electronic density of states (DOSs). (a) DOSs for bulk $NiPS_3$ at 20 GPa. (b) DOSs for monolayer $NiPS_3$ at 20 GPa.

**References**

[1] M. Bernasconi, G. L. Marra, G. Benedek, L. Miglio, M. Jouanne, C. Julien, M. Scagliotti, and M. Balkanski, Phys. *Lattice dynamics of layered MPX,* Rev. B **38**, 12089 (1988).

[2] Y. M. Wang *et al.*, *Raman scattering study of magnetic layered $MPS_3$ crystals (M = Mn, Fe, Ni)*, Chin. Phys. B **28**, 056301 (2019).
